# Supplementary material for: Diffusion in liquid metals is directed by competing collective modes
Source: arXiv:2412.01567 source file (2024-12-02)
Supplement: Supplementary file 1 [file diffpaper_sm.pdf]

# Diffusion in liquid metals is directed by competing collective modes

Franz Demmel*

*ISIS Facility, Rutherford Appleton Laboratory, Didcot, OX11 0QX, UK*

Noel Jakse

*Univ. Grenoble Alpes, CNRS, Grenoble INP, SIMaP, F-38000 Grenoble, France*

## SUPPLEMENTAL MATERIAL

### Assessment of the derived potentials

The ab-initio molecular dynamics simulations were mainly taken from [1, 2] and extended to the undercooled region. For the sake of self-consistency, we recall here the main technical details. The simulations of liquid Al were performed by means of the Vienna Ab initio Simulation Package (VASP) [3]. The local density approximation [4, 5] within projected augmented plane-waves [6] was applied to all simulations with a plane-wave cutoff of 241 eV. Only the $\Gamma$ point is used to sample the Brillouin zone. $N = 256$ atoms are placed in a cubic simulation box of volume $V$ with standard periodic boundary conditions. Newton's equations of motion were solved numerically with Verlet's algorithm in the velocity form with a time step of 1.5 fs, and phase-space trajectories were constructed within the canonical ensemble ($NVT$), by means of a Nosé thermostat to control the temperature $T$. We have shown that all these approximations reproduce the structural and transport properties of Al correctly [1]. For each temperature, the simulation cell was resized according to the experimental density and the run was continued for 30 ps before performing the next quench, resulting in an average cooling rate of $3.3 \cdot 10^{12}$ K/s. Figure 1 shows a comparison between the ab initio simulated diffusion coefficients with the values from the machine learned potential. The perfect agreement demonstrates the reliability of our potential description in relation to the diffusion coefficients over a very wide temperature range.

### Additional results for liquid Rb

Fig 2 displays the VACF for liquid Rb for 4 temperatures. With increasing temperature the negative part diminishes. To quantify the changes a time integral was calculated: $\int_{0.18}^{1.8} \psi(t)dt$. The inset shows the resulting integral against temperature. Around T=500 K the integral becomes positive, signalling the backscattering effect is weakening. In Fig. 3 the diffusion coefficients of liquid Rb are plotted on a logarithmic scale against the inverse temperature. Included as a line is an Arrhenius-type fit between $T_m$ and 1.4 $T_m$. An Arrenhius-type process describes the diffusion coefficients very well within this temperature range. At higher temperatures D deviates to larger values than expected from the Arrhenius process. The data point start to deviate at around $T \approx 1.4T_m$. At the lowest temperature

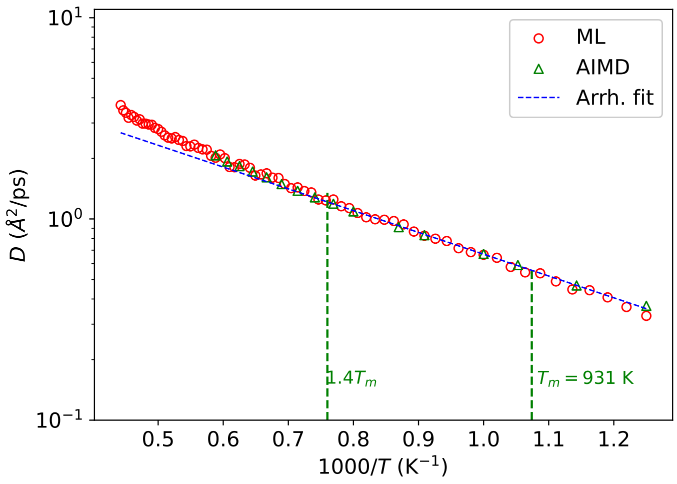


FIG. 1. Diffusion coefficients for liquid Al are presented on a logarithmic scale against the inverse temperature derived from the ab initio simulation in comparison with the machine learned potential results. Included is an Arrhenius-type fit between $T_m$ and 1.4 $T_m$ evidencing the change in dynamics with rising temperature.

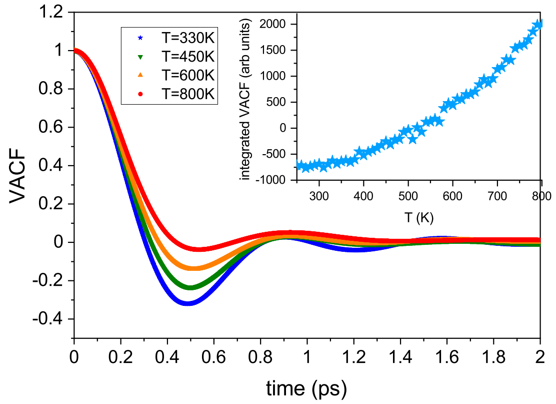


FIG. 2. The normalized VACF is presented for liquid Rb with rising temperature. The inset shows the time integrated VACF between 0.18 ps and 1.8 ps for Rb.

the diffusion coefficient decreases below the Arrhenius line expected values towards structural arrest.

The inset in figure 3 shows the diffusion coefficients against the excess entropy $S_{ex}$ on a logarithmic scale for liquid Rb. The fitted line for entropy values corresponding to temperatures between $T_m$ and 1.4 $T_m$ indicates a good agreement for a wide range in temperatures.

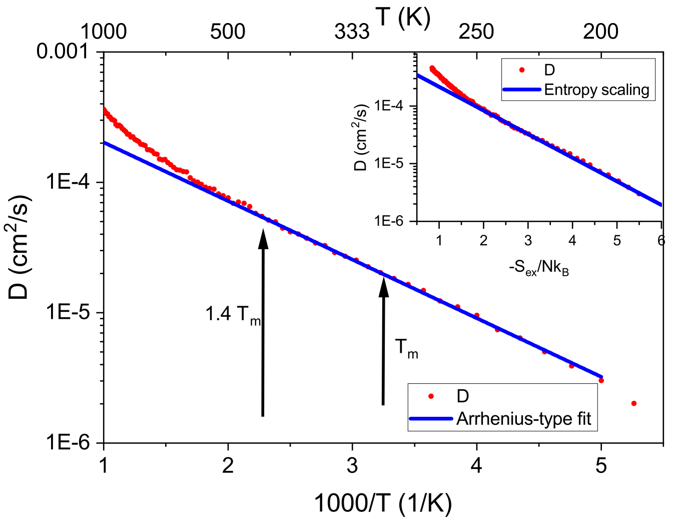


FIG. 3. The diffusion coefficients of Rb are plotted on a logarithmic scale against the inverse temperature. Included is an Arrhenius-type fit between $T_m$ and 1.4 $T_m$ (line). The inset shows $D$ for Rb on a logarithmic scale as a function of the reduced negative excess entropy. The line corresponds to a fit with $D\ \exp(-S_{ex}/Nk_B)$ in the range between $T_m$ and 1.4 $T_m$.

At high temperatures, corresponding to the small negative excess entropy values, the diffusion coefficients deviate from the exponential scaling law.

### Assessment of the Arrhenius fitting procedure

In order to determine the range of the Arrhenius behavior above the melting point, we started with a first regression in a fitting range between $T_m$ and $1.2T_m$ (to have a meaningful regression), and performed iteratively new regressions by adding each time one D value at higher temperature up to the last point, namely at the highest temperature. The left panel of Figs. 4 and 5, respectively for Al and Rb, shows the evolution of the Arrhenius fits with increasing fitting range (from blue to yellow color). The respective right panel corresponds to the $\chi^2$ goodness of fit for each Arrhenius model as a function of the upper limit of the fitting range, while the inset shows the evolution of the Root-Mean-Square Error (RMSE). For both metals, increasing the fitting range from $[T_m,\ 1.2T_m]$ to $[T_m, 1.4T_m]$ does not change the goodness of fit, which takes the lowest value. The same applies to the RMSE. Increasing further the upper bound of the fitting range leads to a progressive degradation of the goodness of fit (higher $\chi^2$ values) and corresponding RMSE, indicating that the data

progressively depart from an Arrhenius behavior above 1.4 $T_m$.

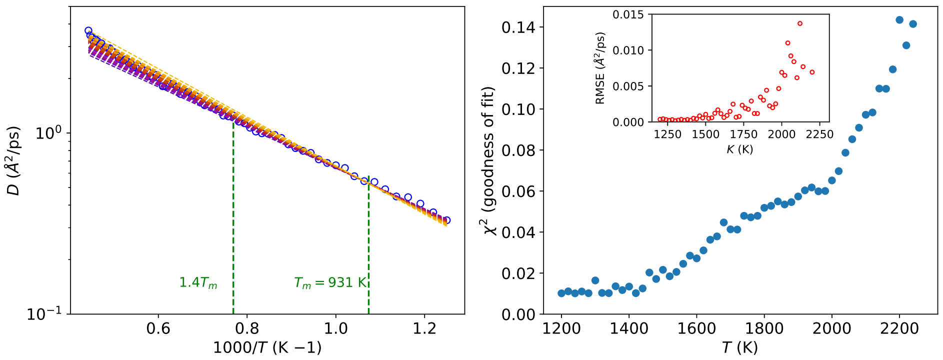


FIG. 4. (Left panel) Arrhenius plot of the diffusion for Al. The open circles represent the simulated values of the diffusion coefficients and the dashed lines correspond to the various Arrhenius fits. (Right panel) $\chi^2$ goodness of the fit for each Arrhenius fitting, as described in the text. The inset represents the RMSE evaluated with respect to the simulated data in the same fitting range).

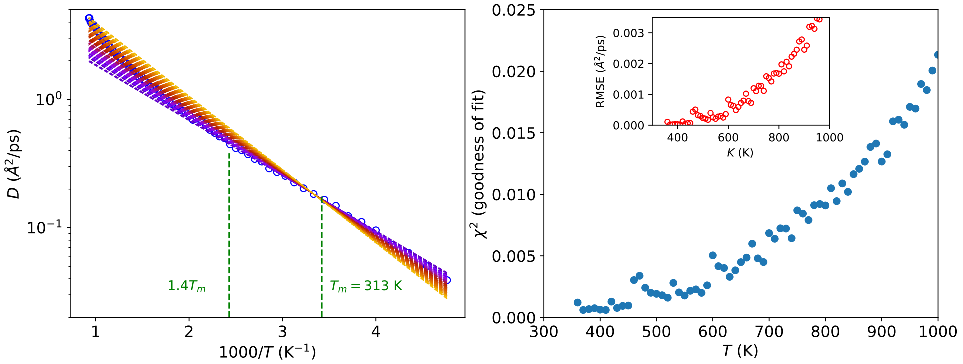


FIG. 5. (Left panel) Arrhenius plot of the diffusion for Rb. The open circles represent the simulated values of the diffusion coefficients and the dashed lines correspond to the various Arrhenius fits. (Right panel) $\chi^2$ goodness of the fit for each Arrhenius fitting, as described in the text. The inset represents the Root-Mean-Square Error (RMSE) evaluated with respect to the simulated data in the same fitting range.

* franz.demmel@stfc.ac.uk

[1] N. Jakse, A. Pasturel, Dynamic properties of liquid and undercooled aluminium. J. Phys. Condens Matter **25** 28510 (2013).

[2] N. Jakse, A. Pasturel, Interplay between structural and atomic transport properties of undercooled Al-Cu binary alloys. AIP Advances **7** 105212 (2017).

[3] G. Kresse, J. Furthmuller, Efficiency of ab-initio total energy calculations for metals and semiconductors using a plane-wave basis set. Comput. Mater. Sci. **6** 15–46 (1996).

[4] D.M. Ceperley, B.J. Alder, Ground State of the Electron Gas by a Stochastic Method. Phys. Rev. Lett. 45, 566–569 (1980).

[5] J.P. Perdew, A. Zunger, Self-interaction correction to density-functional approximations for many-electron systems. Phys. Rev. B 23, 5048–5079 (1981).

[6] G. Kresse, D. Joubert, From ultrasoft pseudopotentials to the projector augmented-wave method. Phys. Rev. B **59** 1758–1775 (1999).
